# Supplementary material for: Persistent Charge Density Wave Memory in a Cuprate Superconductor
Source: arXiv:1807.09066 ancillary file (2018-07-25)
Supplement: Supplementary file 1 [file supplementary.pdf]

# Supplementary Information

(Dated: July 25, 2018)

Here we present details of the data processing for the cross-correlation calculations (Sec. S1), a simulation describing the behavior of the speckles seen in Fig. 2 of the main text (Sec. S2) and a measurement of the LTO domain size (Sec. S3).

## S1. DATA ANALYSIS

In this section, we discuss the background treatment of the raw speckle data in order to obtain Fig. 3(g) in the main text and the fitting procedure to determine the onset of the transition.

Our approach is similar to that used in previous x-ray speckle measurements of magnetic domains [1–3]. In our experiment, Cu $L_3$-edge resonant coherent scattering from LBCO 1/8 has three components: fluorescent background, the overall charge density wave (CDW) Bragg peak, and speckles arising from interference between different CDW domains [4, 5]. (See Fig. 2 of Ref [4] for an illustration of the decomposition of the different peak components.) The cross-correlation of two matrices $A$ and $B$ of size $M \times N$ is defined in Eq. 1 of the main text. Since $A$ and $B$ are 2D matrices, so is the result of the cross-correlation. In our calculation, we chose $A$ (the matrix before the temperature cycle) and $B$ (the matrix after the temperature cycle) to be $200 \times 200$ detector pixels, corresponding to the central area of the CDW peak. Example data measured at 24 K after cycling to $T_{\text{cycle}} = 224$ K is shown in Fig. S1(a)&(b). The cross-correlation of the raw images (Fig. S1(a)&(b)) is plotted in Fig. S2(a), which is dominated by a triangular-shape resulted from fluorescent background and the overall CDW Bragg peak on top of the speckle signals. The triangular shape is more visible with a vertical line-cut plotted as the blue line in Fig. S2(c). In order to isolate speckles from background and incoherent CDW peak, we subtracted a smoothed envelope (*i.e.* $A^* = A - S(A)$, where $S$ is a smoothing function) from raw $A$ and $B$. Fig. S2 (b), and its line-cut in (c, green) displays the effect of this speckle isolation. This data treatment is necessary such that the cross-correlation calculation represents the

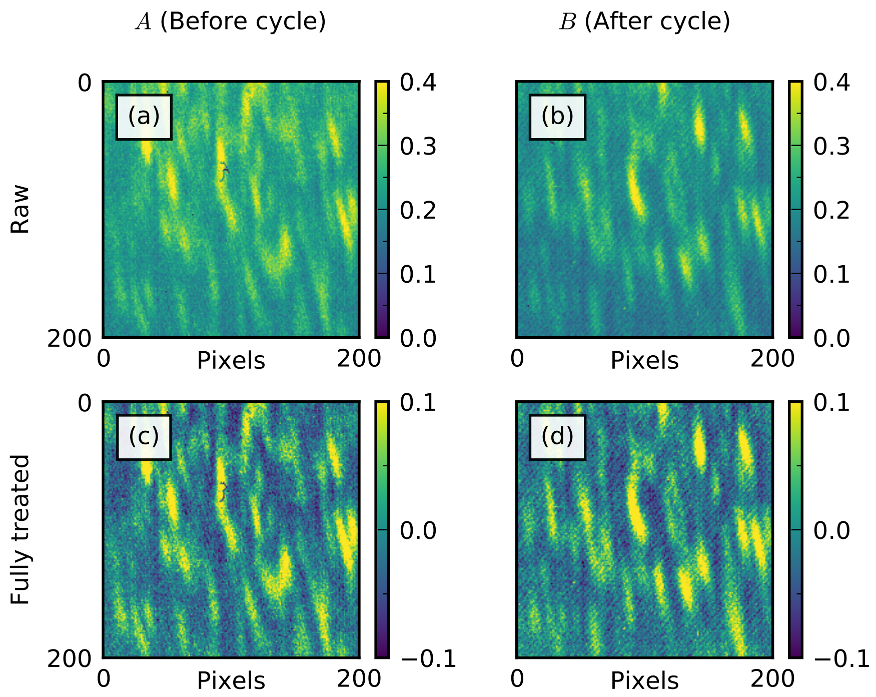


FIG. S1. Example raw and treated data taken at 24 K before and after a temperature cycle to $T_{\text{cycle}} = 224$ K corresponding to matrices $A$ and $B$. (a)&(b) Raw data (a) before and (b) after the temperature cycle in units of photons/s. (c)&(d) Data after treatment (c) before and (d) after the temperature cycle.

reproducibility of the CDW domains independent overall background. For completeness we show the treated detector images in Fig. S1(c)&(d).

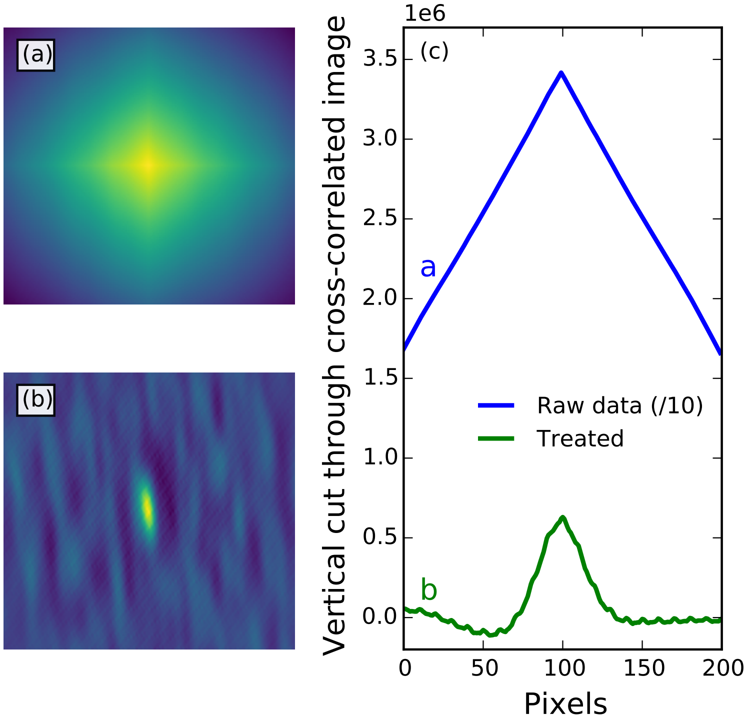


FIG. S2. (a),(b) Cross-correlation matrices of (a) raw data, (b) smoothed background subtracted fully treated data. (c) Vertical line cuts through the cross-correlation matrices in (a) and (b).

After calculating the normalized cross-correlation coefficients for all the data points in Fig. 3(g) (main text), we used an error function

$$\mathrm{erf}\,(x) = \frac{a}{\sqrt{\pi}} \int_0^{\frac{-(x-b)}{d}} e^{-t^2} dt + \frac{1}{2} + c \tag{S1}$$

to fit the shape of the transition. In this form, $a$, $b$, $c$ and $d$ are the step amplitude, center, offset and width, respectively. The $t$ parameter is a dummy variable that is integrated out of the final form. The constants are chosen such at erf($x$) is a step function from 1 to 0 when $a = 1$, $b = 0$, $c = 0$ and $d \to 0^+$. We define the onset temperature of the transition as the intercept of two linear lines extrapolated from the slopes of the error function before and at the center-point of the transition, as shown in Fig. S3. We note that the height of the fit line on the left hand side of the plot may appear too low upon initial inspection, but that this is due to the low values of the cross correlation at $T_{\mathrm{cycle}} = 223.6$ and 223.7 K, which fall well below the fit line.

## S2. SIMULATION OF DOMAIN BEHAVIOR

In Fig. 2 (main text), we saw persistent speckle positions when the temperature was varied in the LTT phase. This observation might not be immediately intuitive because the average CDW domain size decreases with increasing temperature as seen in Fig. S4, so one might have expected to see a change in the speckle pattern. In this section, we calculate the speckle patterns of a simple artificial domain configurations to understand our observation. In the simulation, 500 domains were created at random positions within a circular area of diameter 600 pixels that represents the pinhole in the experiment. Each domain $i$ at location $(x_i, y_i)$ was represented by a 2d Gaussian function

$$g(x, y) = \frac{1}{\sigma\sqrt{2\pi}} \exp\left(-\frac{(x - x_i)^2 + (y - y_i)^2}{2\sigma}\right) \tag{S2}$$

where $\sigma$ is the domain size. In this section, we compare the speckle patterns that arise from domain configurations with the same domain locations, but different domain sizes. Figure S5 displays the result, in which a zoomed area

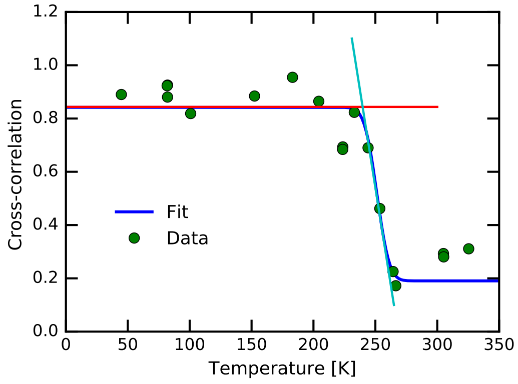


FIG. S3. Determination of the decorrelation onset temperature. Two lines are extrapolated from the low temperature limit and the midpoint of the error function. The onset is defined as the intersection of these two lines.

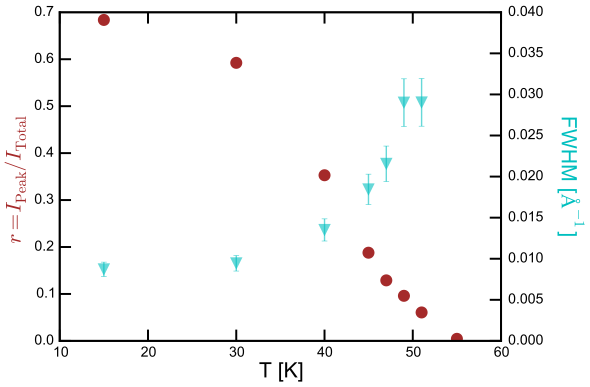


FIG. S4. The ratio of CDW peak intensity to the total intensity (brown circles, left axis) and FWHM (cyan inverted triangles, right axis) as a function of temperature obtained from fitting a Lorentzian-squared line shape to line cuts through the peak. Data were obtained from the same sample that we studied in the present paper [4].

of 100 $\times$ 100 pixels is shown. Panel (a) shows the initial configuration in which the domains were randomly assigned sizes of $\sigma = 4 \pm 2$ pixels. We found that very similar speckle locations are generated even if the domain size is doubled to $\sigma = 8 \pm 4$ as illustrated in Fig. S5(b)&(e). The difference in the speckle pattern with increasing domain size occurs mainly in the shape and distribution of the speckles, rather than their locations. This symmetric expansion of domains about the same locations explains the phenomenology seen in Fig. 2 (main text) where similar speckle patterns are seen despite a factor two change in correlation length as seen in Fig. S4. This applies up to the point at which domains merge as seen by the different pattern in Fig. S5(e)&(f). We note that in diffraction we only see one of two possible domains, so one does not necessarily expect to see merging domains, which will in any case be suppressed as adjacent CDW domains may have different phases.

## S3. SIZE OF LOW-TEMPERATURE ORTHORHOMBIC (LTO) DOMAINS

In view of the relationship between the LTO and CDW domains, we measured the average LTO domain size by x-ray diffraction. A small crystal fragment of the same LBCO 1/8 sample was taken to the 34-ID-C beamline of the Advanced Photon Source (APS). A portable cryostat was used to cool the sample into the low-temperature orthorhombic (LTO) phase at 140 K and the $(\frac{1}{2}\frac{1}{2}2)_{\text{HTT}}$ (or $(012)_{\text{LTO}}$) reflection was located on a Timepix detector with $p = 55$ $\mu$m pixels placed $D = 2.2$ m away. Because the 9 keV beam ($\lambda = 0.137$ nm) was coherent, the crystal was rocked in $\theta$ through the peak and the middle 30 frames (0.001° step size) were averaged together to smooth out the fringes. Radial and transverse cross sections were made through the detector diffraction pattern to extract the peak widths as shown in Fig. S6.

The radial FWHM is 6 pixels wide, corresponding to an LTO domain size of $\lambda D/6p = 920$ nm along the $(\frac{1}{2}\frac{1}{2}2)_{\text{HTT}}$

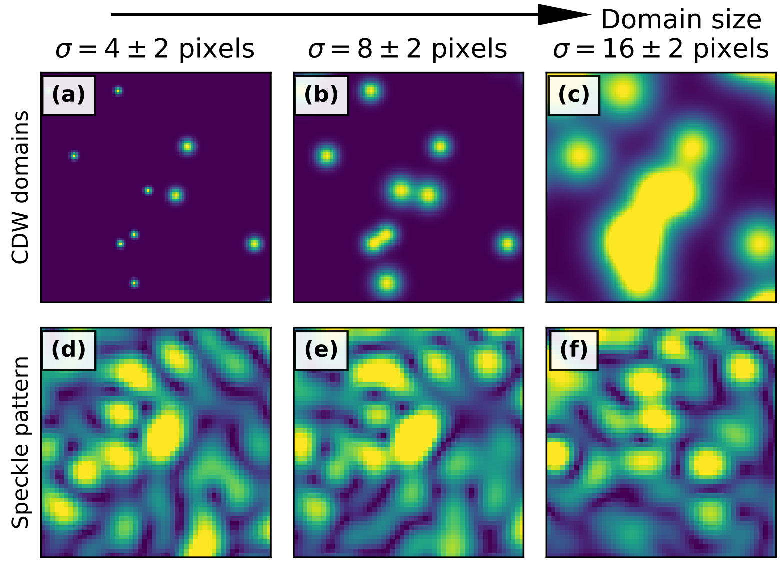


FIG. S5. Simulation of speckle pattern behavior, based on the uniform expansion of domains about the same locations. (a)-(c) Real space domain configurations. A zoomed area of 100 × 100 pixels is shown. The average domain size is doubled from (a) to (b). In (c), domains start to merge into each other. (d)-(f) Speckle patterns for the images in the first row obtained from the Fourier transform squared. A zoomed area of 100 × 100 pixels located 175 pixels away from the peak-center is shown.

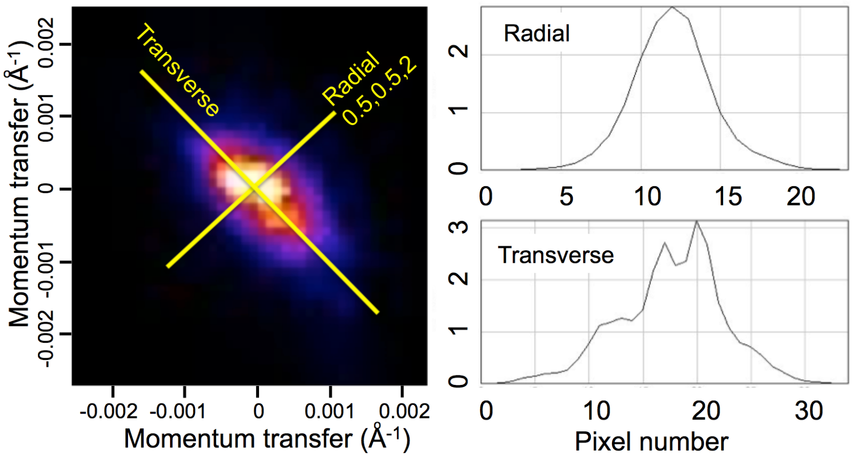


FIG. S6. Determination of LTO domain sizes. Left: Diffraction pattern of the $(\frac{1}{2}\frac{1}{2}2)_{\rm HTT}$ or $(012)_{\rm LTO}$ peak measured on a Timepix area detector. Right: profiles of the peak in the radial and transverse directions.

direction. The transverse FWHM is 13 pixels wide, giving a domain size of 420 nm. From the $\Delta\theta = 0.06°$ FWHM width of the $\theta$-scan (not shown), the domain size is $\lambda/2\sin\theta\Delta\theta = 400$ nm along the out-of-detector-plane direction. Here we take the average values of 700 nm as a typical LTO domain size. This number agrees well with the TEM observations [6, 7].

[1] Michael S Pierce, Rob G Moore, Larry B Sorensen, Stephen D Kevan, Olav Hellwig, Eric E Fullerton, and Jeffrey B Kortright, "Quasistatic X-Ray Speckle Metrology of Microscopic Magnetic Return-Point Memory," Phys. Rev. Lett. **90**, 175502–175504 (2003).

[2] K. Chesnel, J. Nelson, B. Wilcken, and S. D. Kevan, "Mapping spatial and field dependence of magnetic domain memory by soft X-ray speckle metrology," Journal of Synchrotron Radiation **19**, 293–306 (2012).

[3] Karine Chesnel, Alex Safsten, Matthew Rytting, and Eric E Fullerton, "Shaping nanoscale magnetic domain memory in exchange-coupled ferromagnets by field cooling," Nature Communications **7**, 11648 (2016).

[4] X. M. Chen, V. Thampy, C. Mazzoli, A. M. Barbour, H. Miao, G. D. Gu, Y. Cao, J. M. Tranquada, M. P. M. Dean, and S. B. Wilkins, "Remarkable stability of charge density wave order in $La_{1.875}Ba_{0.125}CuO_4$," Phys. Rev. Lett. **117**, 167001 (2016).

[5] V Thampy, XM Chen, Y Cao, C Mazzoli, AM Barbour, W Hu, H Miao, G Fabbris, RD Zhong, GD Gu, *et al.*, "Static charge-density-wave order in the superconducting state of $La_{2-x}Ba_xCuO_4$," Phys. Rev. B **95**, 241111 (2017).

[6] Yimei Zhu, A. R. Moodenbaugh, Z. X. Cai, J. Tafto, M. Suenaga, and D. O. Welch, "Tetragonal-orthorhombic structural modulation at low temperature in $La_{2-x}Ba_xCuO_4$," Phys. Rev. Lett. **73**, 3026–3029 (1994).

[7] Y Horibe, Y Inoue, and Y Koyama, "Direct observation of dynamic local structure in $La_{2-x}Sr_xCuO_4$ around $x = 0.12$," Physical Review B **61**, 11922 (2000).
